# Supplementary material for: Phrase Retrieval Learns Passage Retrieval, Too
Source: arXiv:2109.08133 source file (2021-09-16)
Supplement: Supplementary file 1 [file appendix.tex]

    %!TEX root = ../main.tex

\clearpage
\section{Encoding Phrase Representations}\label{sec:apdx1}

\label{sec:appendix}
